# Supplementary material for: Tree Prompting: Efficient Task Adaptation without Fine-Tuning
Source: arXiv:2310.14034 source file (2023-10-21)
Supplement: Supplementary file 1 [file appendix.tex]

\appendix
\counterwithin{figure}{section}
\counterwithin{table}{section}

\section{Appendix}
